# Supplementary material for: Deconstructing the Blockchain to Approach Physical Limits
Source: arXiv:1810.08092 source file (2019-10-02)
Supplement: Supplementary file 1 [file latency_appendix_proofs.tex]

\section{Appendix: Proofs of Lemmas used in Appendix \ref{appen:sec:latency_proof}}
