# Supplementary material for: Deconstructing the Blockchain to Approach Physical Limits
Source: arXiv:1810.08092 source file (2019-10-02)
Supplement: Supplementary file 2 [file related_appendix.tex]

\section{Analysis of Related Work}
\label{app:related}

\subsection{Bitcoin}
\label{app:bitcoin}
\input{bitcoin}

\subsection{Bitcoin-NG}
\label{app:bitcoin-ng}

\subsection{GHOST}
\label{app:ghost}
\input{ghost.tex}

\subsection{Conflux}
\label{app:conflux}

\subsection{Phantom}
\label{app:phantom}
